# Supplementary material for: Spatial Language Representation with Multi-Level Geocoding
Source: arXiv:2008.09236 source file (2020-08-21)
Supplement: Supplementary file 1 [file appendix.tex]

\section*{Appendix}

% \begin{table*}
%     \centering
%     \begin{tabular}{l|rrr|rrr|rrr}
% & \multicolumn{3}{c|}{WikToR} & \multicolumn{3}{c|}{LGL}  & \multicolumn{3}{c}{GeoVirus}  \\ 
% Model & acc & auc & mean & acc & auc & mean & acc & auc & mean \\
% \hline
% \camcoder & 65 & 33 & 1074 & 75 & 22 & 807 & 81 & 31 & 328 \\
% \ourcamcoder & 68 & 30 & 1063 & 58 & 42 & 954 & 65 & 36 & 552 \\
% \mageIII & 85 & 20 & 823 & 75 & 24 & 686 & 79 & 33 & 512 \\
%     \end{tabular}
%     \caption{Comparing performance with unaltered evaluation sets.} \label{tab:nofix_evals}
% \end{table*}

\begin{table*}
\small
    \centering
    \begin{tabular}{l|rrr|r||rrr|r||rrr|r}
 & \multicolumn{4}{c||}{AUC of error curve} & \multicolumn{4}{c||}{accuracy@161}  & \multicolumn{4}{c}{Mean error}  \\ 
Model & WTR & LGL & GeoV & Avg & WTR & LGL & GeoV & Avg & WTR & LGL & GeoV & Avg \\
\hline
\camcoder & 33 & 22 & 31 & 29 & 65 & 75 & 81 & 74 & 1074 & 807 & 328 & 736 \\ 
\ourcamcoder & 30 & 42 & 36 & 36 & 68 & 58 & 65 & 64 & 1063 & 954 & 552 & 856 \\ 
\mageIII & 20 & 24 & 33 & 26 & 85 & 75 & 79 & 80 & 823 & 686 & 512 & 674 \\
\end{tabular}
    \caption{Comparing performance with unaltered evaluation sets.} \label{tab:nofix_evals}
\end{table*}

% \paragraph{Unifying the evaluation data}
% Steps on how the patches.tsv was generated \SK{}

\subsection*{Evaluation on unaltered datasets}
For the sake of comparison, we also report performance of \mageIII on the unaltered evaluation sets in Table \ref{tab:nofix_evals}.  Recall also that we retrained \camcoder on our training material and report its performance as \ourcamcoder to minimize differences from training data and focus on modeling choices. There is a large gap between the original and our implementation, with the former performing much better on LGL and GeoVirus, and the latter mildly improved on WiKtoR. The gap is more severe in GeoVirus, since this dataset includes many examples for large regions like China, Canada, etc. which are now standardized to their coordinates as represented in WikiData. We suspect that this is because the original CamCoder's training material included examples from all three toponym resolution datasets as well as harvesting examples from Wikipedia, and that this allowed the model to fit and accommodate the inconsistencies between datasets, in part.

\subsection*{Examples to demonstrate advantage from joint loss}
Table \ref{tab:mlg-examples} shows some examples on how the coarser levels help to nudge the predictions close to the true value. While just including the loss from different levels at training time helps for first two examples, using a joint prediction at inference time gives additional gains as shows in last two examples. This can be attributed to the other locations in the context that represent larger regions -- typically the locations that contain the target location. 

\begin{table*}
    \centering
    \begin{tabular}{p{10.5cm} | p{1cm}p{1.2cm}p{1.2cm}}
\center{Context (partial)} & \small{\mageoneVII (L7)} & \small{\mageIII (L7)} & \small{ \mageIII (L5-7)}  \\
\hline
% XXY
% \textbf{Warren county} is a county located in the U.S. state of Pennsylvania. & X & X & \checkmark \\ \hline
\textbf{Chaoyang} is a prefecture - level city of Liaoning province, People's Republic of China. & X & X & \checkmark \\ \hline
\textbf{Buffalo} is a city, located 40 miles northwest of Minneapolis in Wright county, Minnesota. & X & X & \checkmark \\ \hline

% XYY
\textbf{Buffalo} is a city in Johnson county, Wyoming, United States. & X & \checkmark & \checkmark \\ \hline
\textbf{Lincoln} is a city in Placer county, California, United States, part of the Sacramento metropolitan area.  & X & \checkmark & \checkmark \\% \hline
% \textbf{Bangor} is a city in Van Buren county in the U.S. state of Michigan. & X & \checkmark & \checkmark 
     \end{tabular}
     \caption{Including joint loss in the training objective and in inference helps improve the predictions. Values in the brackets in table header indicate levels used in inference.}
    \label{tab:mlg-examples}
\end{table*}
